# Supplementary material for: Towards Effective User Attribution for Latent Diffusion Models via Watermark-Informed Blending
Source: arXiv:2409.10958 source file (2024-12-16)
Supplement: Supplementary file 1 [file X_suppl.tex]

\setcounter{page}{1}
\maketitlesupplementary

\section{Image Level Attacks.}
Image level attacks aim to eliminate invisible watermarks by modifying the generated images. Perceptual auto-encoders are employed to create compressed latent representations of images, which attackers use to remove the watermarks. In this work, we use the VQ-VAE attack \cite{balle2018variational}, KL divergence attack \cite{ref3}, BMSHJ attack \cite{balle2018variational}, and Cheng attack \cite{cheng2020learned}. The BMSHJ and Cheng attacks are implemented using the CompressAI library zoo, leveraging both the anchor model and the factorized prior model. Specifically, the BMSHJ attack uses compression rates of 1, 4, and 8, while the Cheng attack utilizes compression rates of 1, 3, and 6. Additionally, the VQ-VAE attack is applied with compression rates of 4, 8, and 16. Finally, the KL divergence attack is tested at compression rates of 4, 8, 16, and 32. To evaluate the watermark removal, we generate 1,000 images from text prompts using our watermarked model with a 48-bit key. These images are then processed by the auto-encoders to attempt watermark removal. The bit accuracy of the extracted watermark is computed to measure the attack's effectiveness. Additionally, we calculate the peak signal-to-noise ratio (PSNR) between the original and reconstructed images to quantify the impact on image quality.

For adversarial attacks, we assume that the watermark extractor $\mathcal{D}_w$ is leaked to attackers. The attackers utilize adversarial techniques to replace the original watermark with a random binary message while preserving image quality. This attack is implemented by substituting all training loss terms with the mean squared error (MSE) loss between the extractor's output and the predefined random binary message.
\section{Model Collusion.}
The objective of model collusion is to evaluate the model's resilience when two users average their respective model weights. We fingerprint the decoder with two random watermarks, $m_0$ and $m_1$. Each fingerprinted model is used to generate 500 images, and the extracted bits from these images are compared. When the bits at a given position $j$ in $m_0$ and $m_1$ are the same (either both 1 or both 0), the extracted bit from the colluded model is recorded directly at that position. In cases where the bits at position $j$ differ, the bits are denoted as $m_0^{j}$ and $m_1^{j}$. The average bit value, $m_2$, at position $j$ is calculated as $m_2 = 0.5 * (m_0^{j} + m_1^{j})$. To better illustrate the distribution of the extracted watermark in these cases, we record $m^{j} - m_2$, where $m^{j}$ is the bit extracted from images generated by the colluded model and $m_2$ represents the expected average bit value. We then use Scipy library to fit data, and it is shown in below figure. We have four conditions. The four conditions correspond to the possible combinations of bit values at position $j$ in $m_0$ and $m_1$. $00$: Both $m_0^{j}$ and $m_1^{j}$ are 0. $11$: Both $m_0^{j}$ and $m_1^{j}$ are 1. $01$: $m_0^{j}$ is 0 and $m_1^{j}$ is 1. $10$: $m_0^{j}$ is 1 and $m_1^{j}$ is 0.\par
As illustrated in Fig. \ref{fig:skew}, when the bits at position $j$ in $m_0$ and $m_1$ are the same (00 or 11), the extracted bit from the colluded model aligns closely with these values. Conversely, when the bits differ (01 or 10), the extracted bit exhibits randomness. This randomness is quantitatively analyzed using the deviation $m^{j} - m_2$.
\begin{figure}[h]
    \centering
    \includegraphics[width=0.49\textwidth]{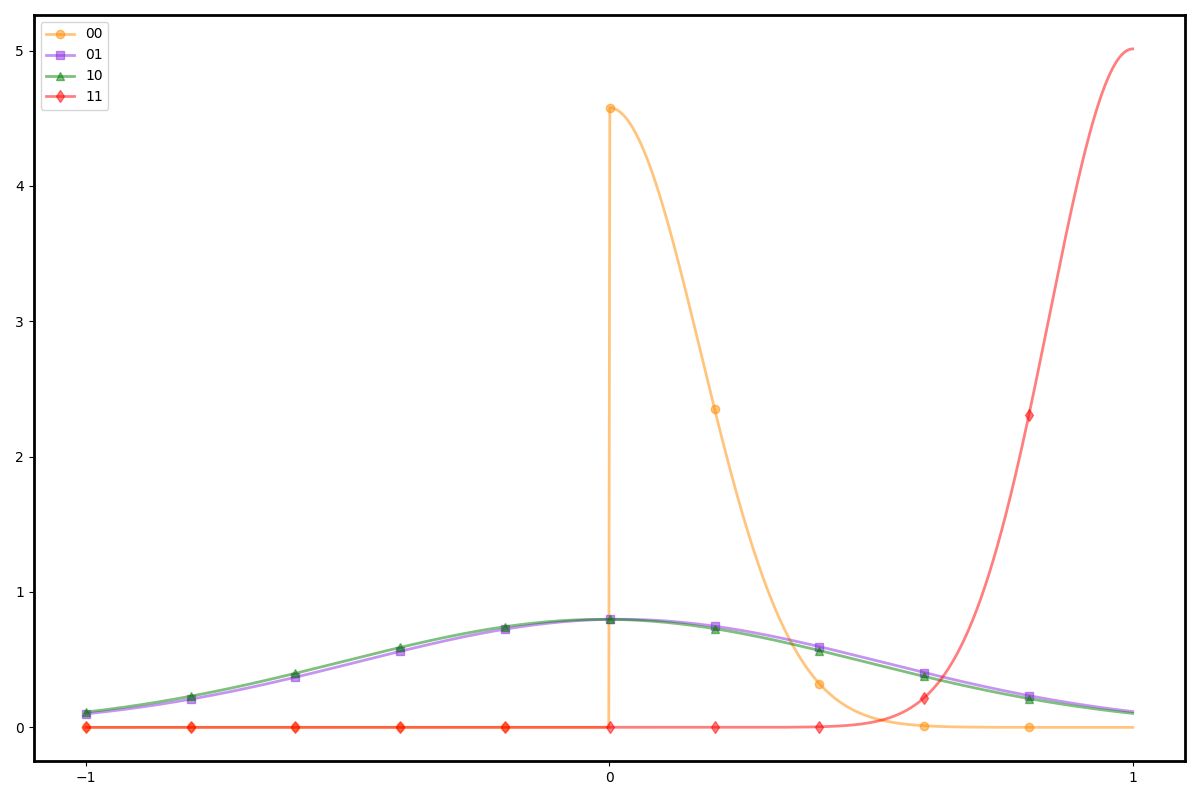}
    \caption{Probability density function of the skewed normal distribution under four conditions. For ''00'' and ''11'', the extracted bit at position $j$ from the colluded model tends to align with the correct bit. Conversely, for ''01'' and ''10'', the extracted bit at position $j$ from the colluded model exhibits randomness.}
    \label{fig:skew}
\end{figure}

\section{Additional Qualitative Results.}
To further demonstrate the effectiveness of our method in enhancing image quality, we provide supplementary qualitative results. Specifically, we include pixel-wise difference images magnified by a factor of 10 to highlight subtle changes. These results compare our method with other merged-in watermarking techniques. As shown in Fig. \ref{fig:1}, \ref{fig:2}, \ref{fig:3}, \ref{fig:4}, \ref{fig:5}, \ref{fig:6}, \ref{fig:7}, our method achieves effective embedding of invisible watermarks while minimizing their impact on image quality. The comparisons illustrate the superiority of our approach in preserving the visual fidelity of the images, even under close inspection.

% Appendix
\newpage

\begin{figure*}[h]
\centering
%\vspace*{0.1cm}
\begin{subfigure}{0.16\textwidth}
\begin{overpic}[width=\linewidth]{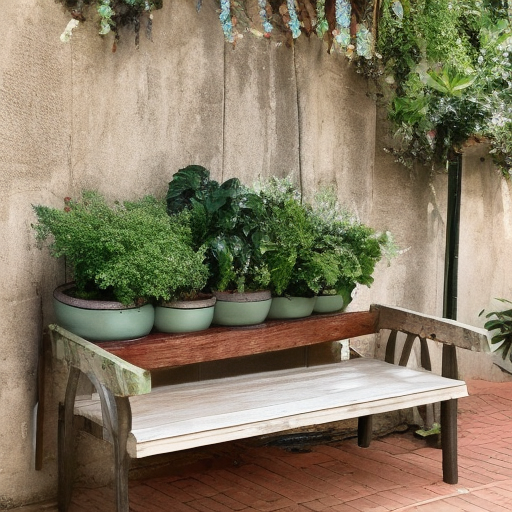}
\put(30,105){\small{Original}} % 文字在上方
\put(-18,40){\rotatebox{90}{\small{SG}}} % 文字在左侧
\end{overpic}
\end{subfigure}
\hfill
\begin{subfigure}{0.16\textwidth}
\begin{overpic}[width=\linewidth]{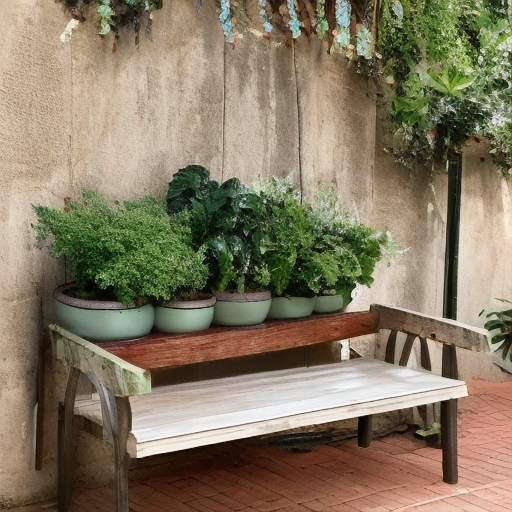}
\put(20,105){\small{Watermarked}}
\end{overpic}
\end{subfigure}
\hfill
\begin{subfigure}{0.16\textwidth}
\begin{overpic}[width=\linewidth]{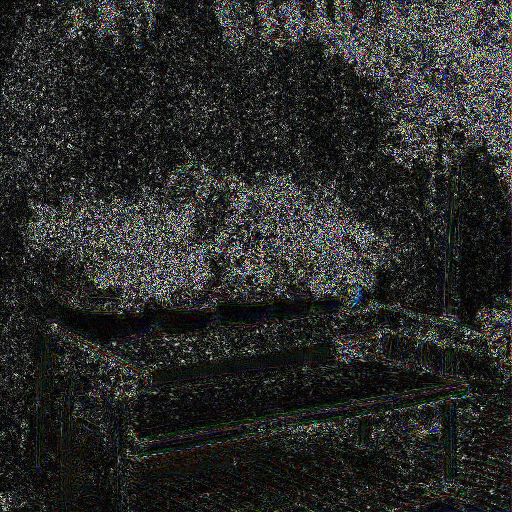}
\put(15, 105){\small{Pixel-wise ($\times$10)}}
\end{overpic}
\end{subfigure}
\hfill
\begin{subfigure}{0.16\textwidth}
\begin{overpic}
    [width=\linewidth]{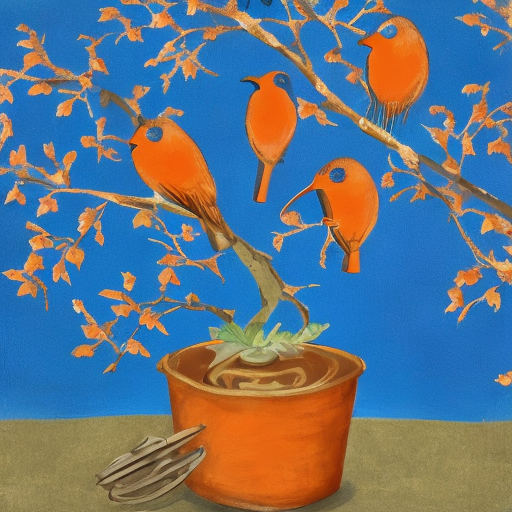}
\put(30,105){\small{Original}}
\end{overpic}
\end{subfigure}
\hfill
\begin{subfigure}{0.16\textwidth}
\begin{overpic}
[width=\linewidth]{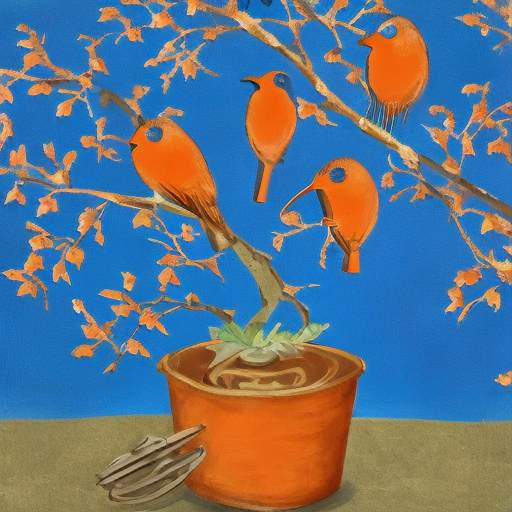}
\put(20,105){\small{Watermarked}}
\end{overpic}
\end{subfigure}
\hfill
\begin{subfigure}{0.16\textwidth}
\begin{overpic}
[width=\linewidth]{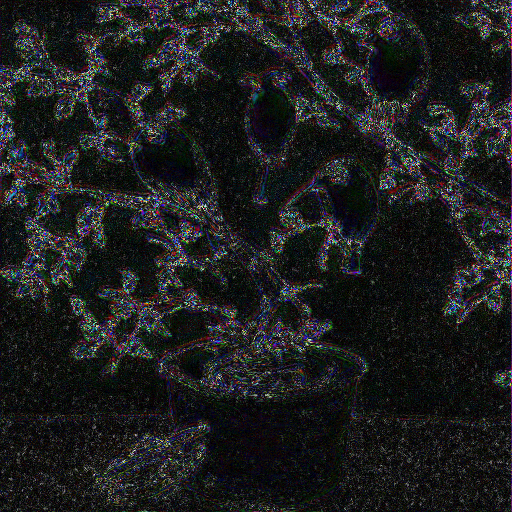}
\put(15, 105){\small{Pixel-wise ($\times$10)}}
\end{overpic}
\end{subfigure}

\begin{subfigure}{0.16\textwidth}
\begin{overpic}[width=\linewidth]{sec/fig/supp/sd/00186.png}
\put(-18,25){\rotatebox{90}{\small{WOUAF}}}
\end{overpic}
\end{subfigure}
\hfill
\begin{subfigure}{0.16\textwidth}
\includegraphics[width=\linewidth]{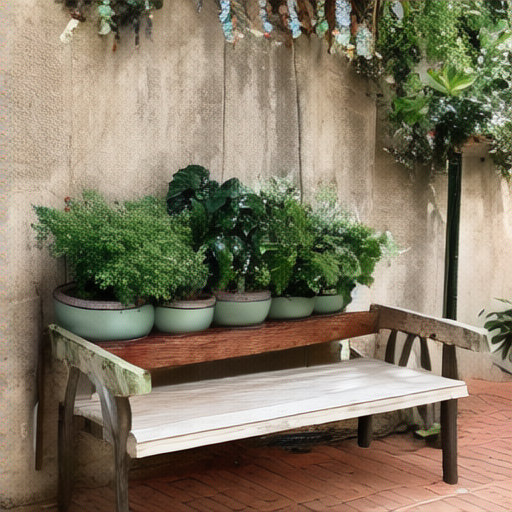}
\end{subfigure}
\hfill
\begin{subfigure}{0.16\textwidth}
\includegraphics[width=\linewidth]{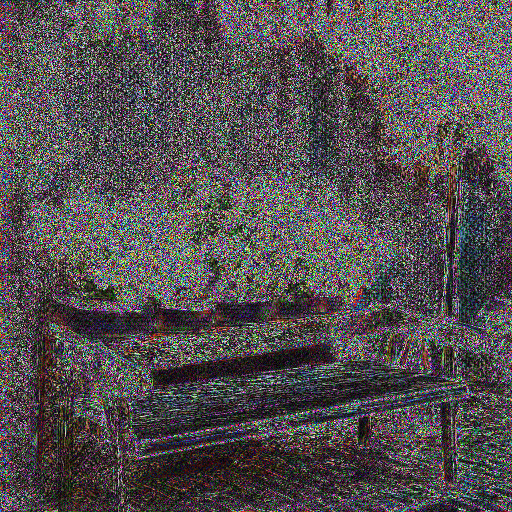}
\end{subfigure}
\hfill
\begin{subfigure}{0.16\textwidth}
\includegraphics[width=\linewidth]{sec/fig/supp/sd/00291.png}
\end{subfigure}
\hfill
\begin{subfigure}{0.16\textwidth}
\includegraphics[width=\linewidth]{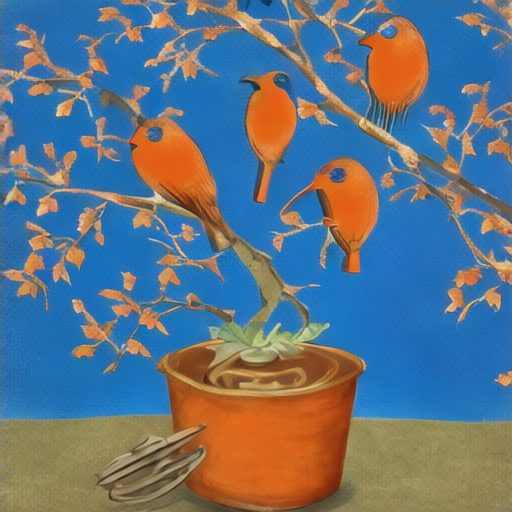}
\end{subfigure}
\hfill
\begin{subfigure}{0.16\textwidth}
\includegraphics[width=\linewidth]{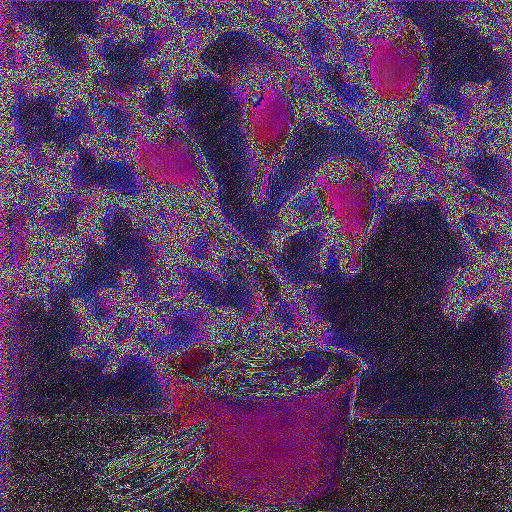}
\end{subfigure}

\begin{subfigure}{0.16\textwidth}
\begin{overpic}
[width=\linewidth]{sec/fig/supp/sd/00186.png}
\put(-18,10){\rotatebox{90}{\small{TEAWIB (ours)}}}
\end{overpic}
\end{subfigure}
\hfill
\begin{subfigure}{0.16\textwidth}
\includegraphics[width=\linewidth]{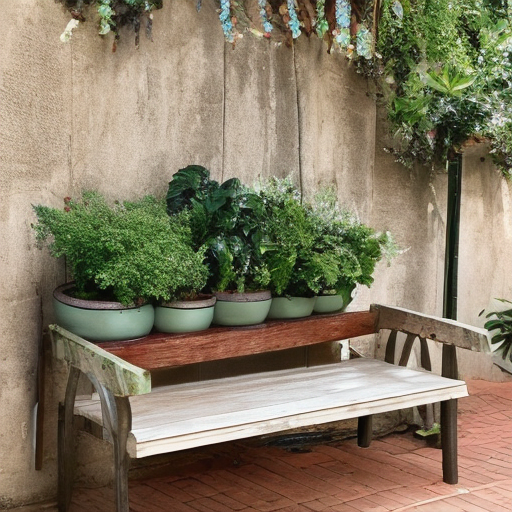}
\end{subfigure}
\hfill
\begin{subfigure}{0.16\textwidth}
\includegraphics[width=\linewidth]{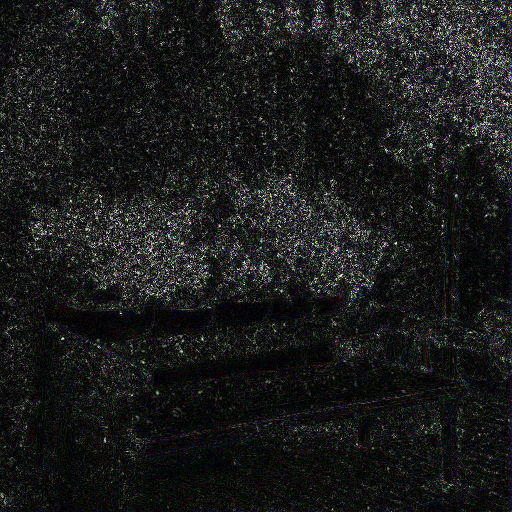}
\end{subfigure}
\hfill
\begin{subfigure}{0.16\textwidth}
\includegraphics[width=\linewidth]{sec/fig/supp/sd/00291.png}
\end{subfigure}
\hfill
\begin{subfigure}{0.16\textwidth}
\includegraphics[width=\linewidth]{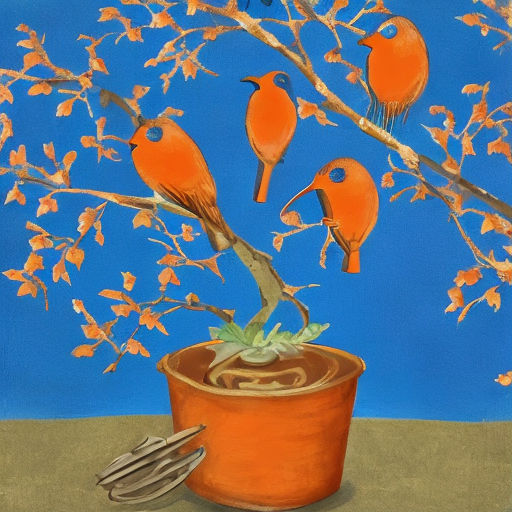}
\end{subfigure}
\hfill
\begin{subfigure}{0.16\textwidth}
\includegraphics[width=\linewidth]{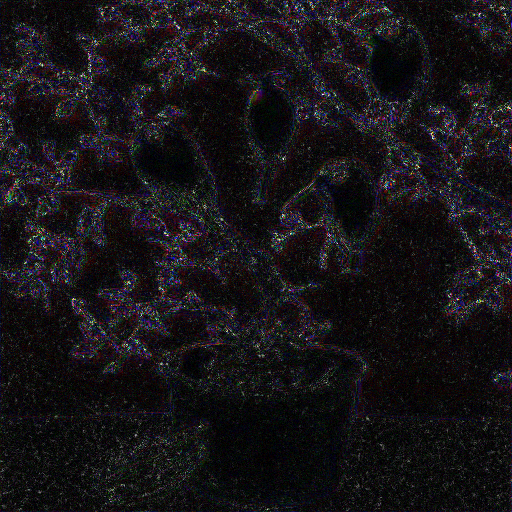}
\end{subfigure}
\caption{Qualitative comparison of TEAWIB with other ad-hoc watermark generation techniques on the MS-COCO validation set. Notably, our method preserves the high quality of the generated image and invisible watermark embedding.}
\label{fig:1}
\end{figure*}

\begin{figure*}[h]
\centering
\vspace*{0.1cm}
\begin{subfigure}{0.16\textwidth}
\begin{overpic}[width=\linewidth]{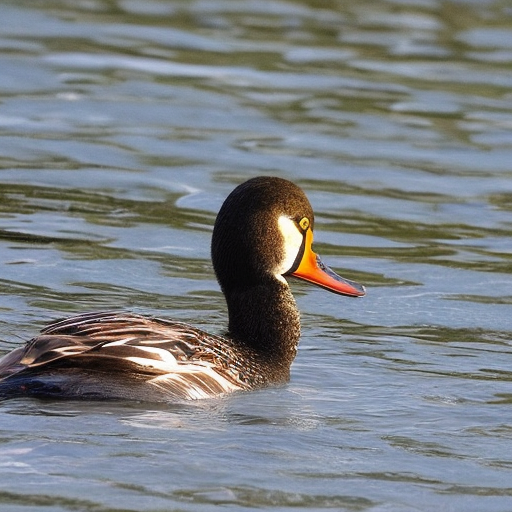}
\put(30,105){\small{Original}} % 文字在上方
\put(-18,40){\rotatebox{90}{\small{SG}}} % 文字在左侧
\end{overpic}
\end{subfigure}
\hfill
\begin{subfigure}{0.16\textwidth}
\begin{overpic}[width=\linewidth]{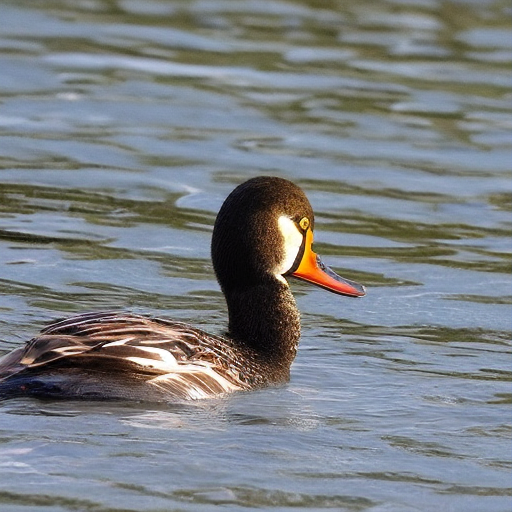}
\put(20,105){\small{Watermarked}}
\end{overpic}
\end{subfigure}
\hfill
\begin{subfigure}{0.16\textwidth}
\begin{overpic}[width=\linewidth]{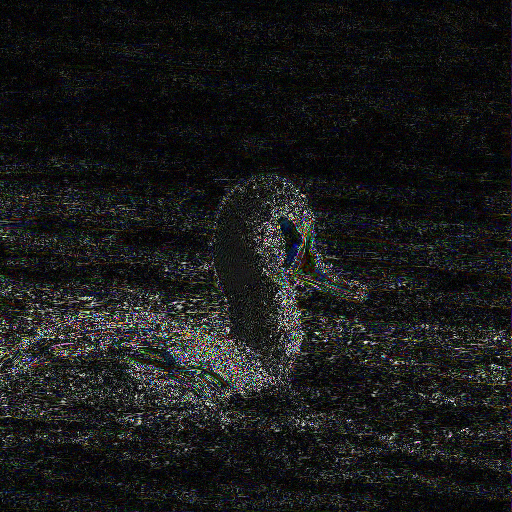}
\put(15, 105){\small{Pixel-wise ($\times$10)}}
\end{overpic}
\end{subfigure}
\hfill
\begin{subfigure}{0.16\textwidth}
\begin{overpic}
    [width=\linewidth]{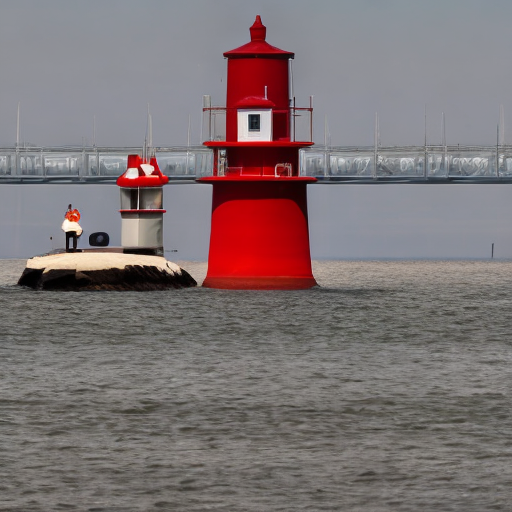}
\put(30,105){\small{Original}}
\end{overpic}
\end{subfigure}
\hfill
\begin{subfigure}{0.16\textwidth}
\begin{overpic}
[width=\linewidth]{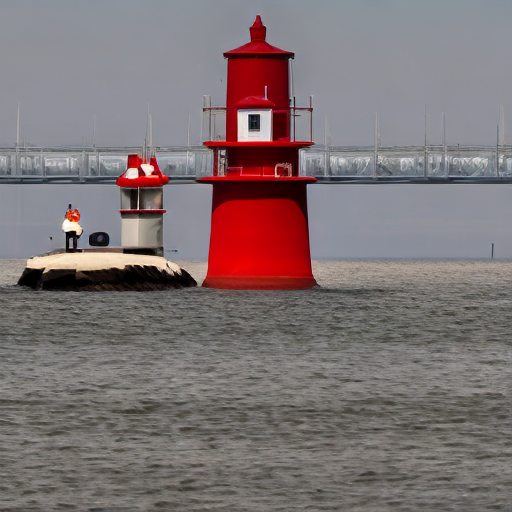}
\put(20,105){\small{Watermarked}}
\end{overpic}
\end{subfigure}
\hfill
\begin{subfigure}{0.16\textwidth}
\begin{overpic}
[width=\linewidth]{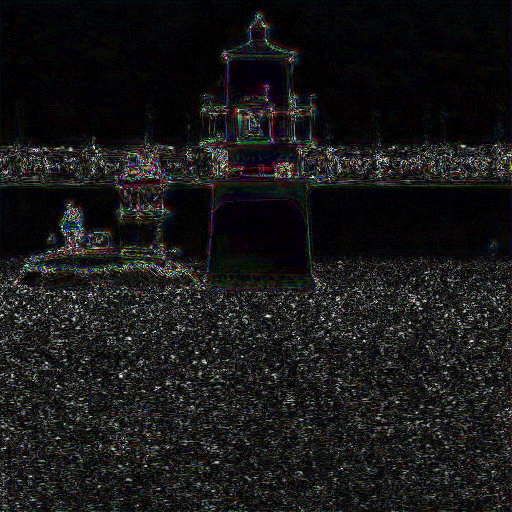}
\put(15, 105){\small{Pixel-wise ($\times$10)}}
\end{overpic}
\end{subfigure}

\begin{subfigure}{0.16\textwidth}
\begin{overpic}[width=\linewidth]{sec/fig/supp/sd/00224.png}
\put(-18,25){\rotatebox{90}{\small{WOUAF}}}
\end{overpic}
\end{subfigure}
\hfill
\begin{subfigure}{0.16\textwidth}
\includegraphics[width=\linewidth]{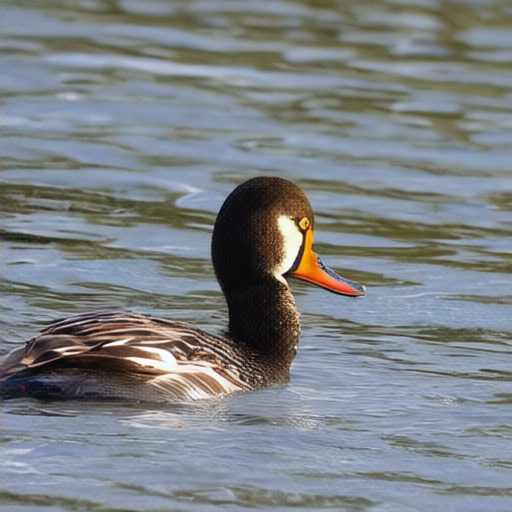}
\end{subfigure}
\hfill
\begin{subfigure}{0.16\textwidth}
\includegraphics[width=\linewidth]{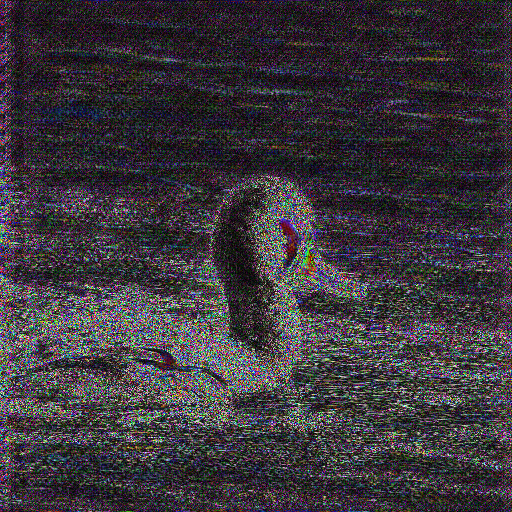}
\end{subfigure}
\hfill
\begin{subfigure}{0.16\textwidth}
\includegraphics[width=\linewidth]{sec/fig/supp/sd/00387.png}
\end{subfigure}
\hfill
\begin{subfigure}{0.16\textwidth}
\includegraphics[width=\linewidth]{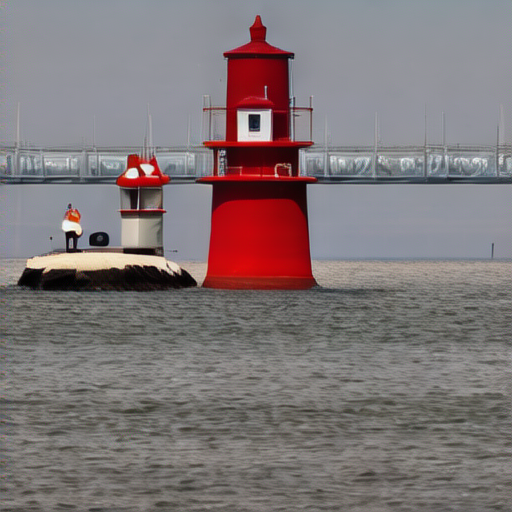}
\end{subfigure}
\hfill
\begin{subfigure}{0.16\textwidth}
\includegraphics[width=\linewidth]{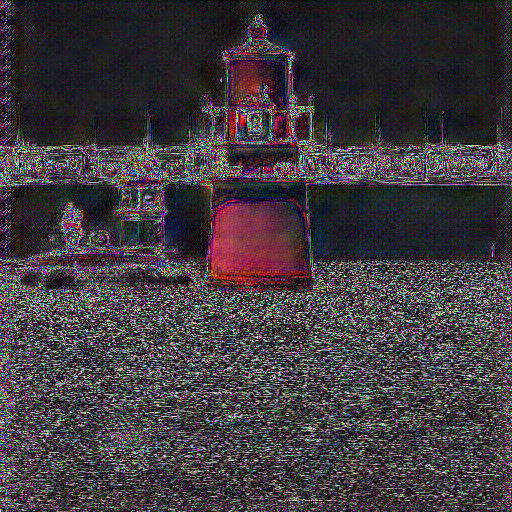}
\end{subfigure}

\begin{subfigure}{0.16\textwidth}
\begin{overpic}
[width=\linewidth]{sec/fig/supp/sd/00224.png}
\put(-18,10){\rotatebox{90}{\small{TEAWIB (ours)}}}
\end{overpic}
\end{subfigure}
\hfill
\begin{subfigure}{0.16\textwidth}
\includegraphics[width=\linewidth]{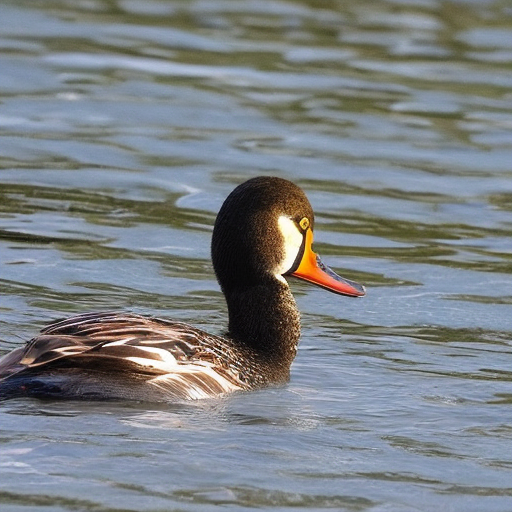}
\end{subfigure}
\hfill
\begin{subfigure}{0.16\textwidth}
\includegraphics[width=\linewidth]{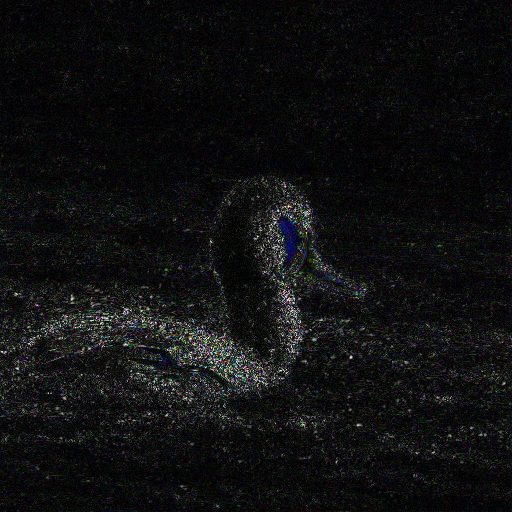}
\end{subfigure}
\hfill
\begin{subfigure}{0.16\textwidth}
\includegraphics[width=\linewidth]{sec/fig/supp/sd/00387.png}
\end{subfigure}
\hfill
\begin{subfigure}{0.16\textwidth}
\includegraphics[width=\linewidth]{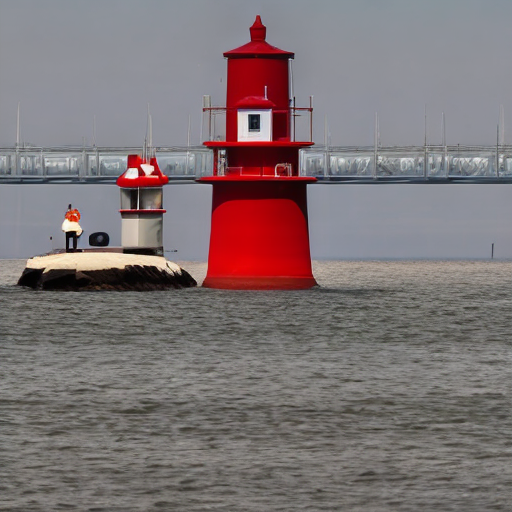}
\end{subfigure}
\hfill
\begin{subfigure}{0.16\textwidth}
\includegraphics[width=\linewidth]{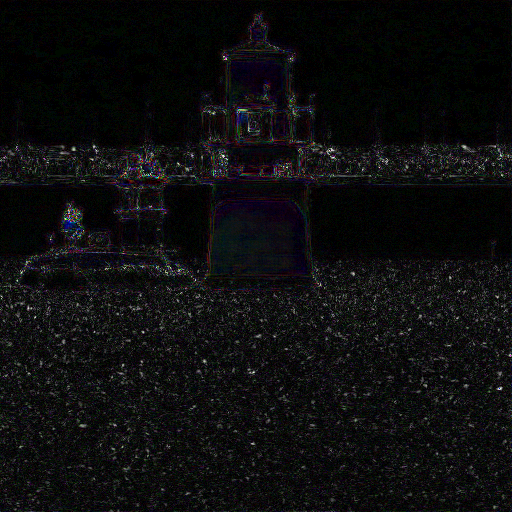}
\end{subfigure}
\caption{Qualitative comparison of TEAWIB with other ad-hoc watermark generation techniques on the MS-COCO validation set. Notably, our method preserves the high quality of the generated image and invisible watermark embedding.}
\label{fig:2}
\end{figure*}

\newpage
\begin{figure*}
\centering
\vspace*{0.1cm}
\begin{subfigure}{0.16\textwidth}
\begin{overpic}[width=\linewidth]{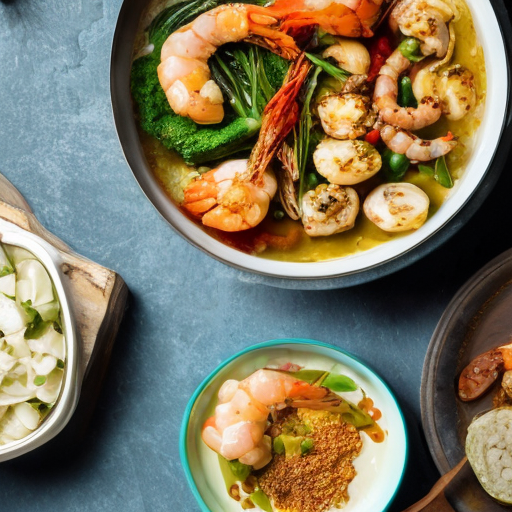}
\put(30,105){\small{Original}} % 文字在上方
\put(-18,40){\rotatebox{90}{\small{SG}}} % 文字在左侧
\end{overpic}
\end{subfigure}
\hfill
\begin{subfigure}{0.16\textwidth}
\begin{overpic}[width=\linewidth]{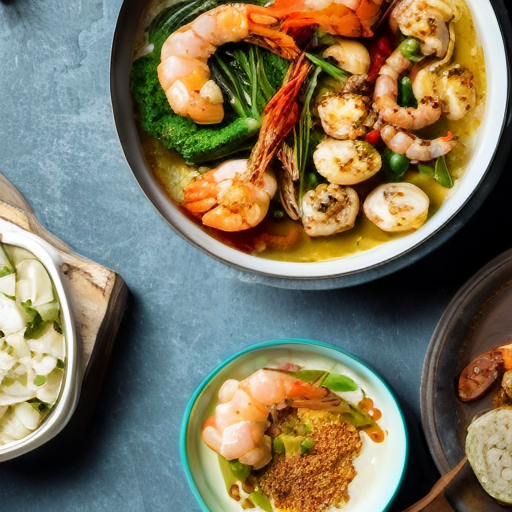}
\put(20,105){\small{Watermarked}}
\end{overpic}
\end{subfigure}
\hfill
\begin{subfigure}{0.16\textwidth}
\begin{overpic}[width=\linewidth]{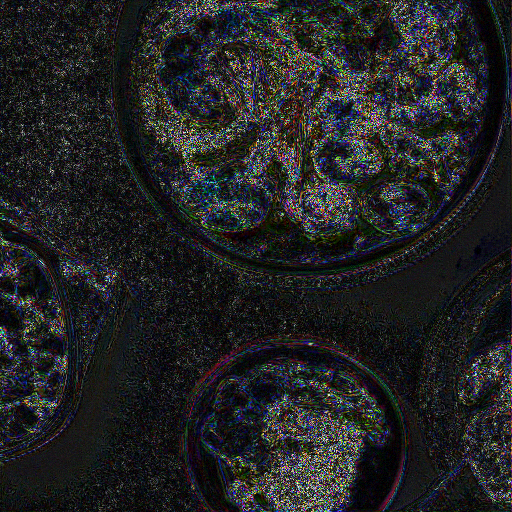}
\put(15, 105){\small{Pixel-wise ($\times$10)}}
\end{overpic}
\end{subfigure}
\hfill
\begin{subfigure}{0.16\textwidth}
\begin{overpic}
    [width=\linewidth]{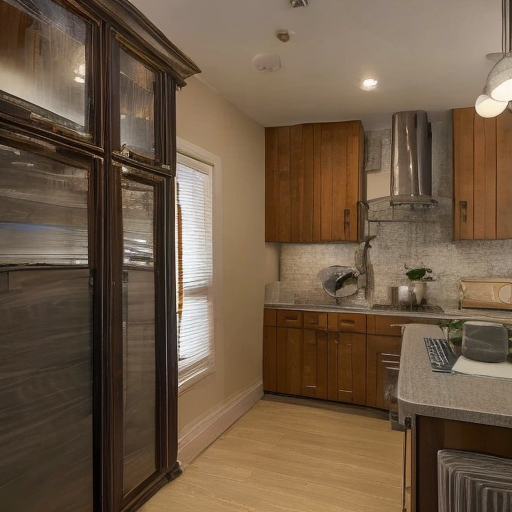}
\put(30,105){\small{Original}}
\end{overpic}
\end{subfigure}
\hfill
\begin{subfigure}{0.16\textwidth}
\begin{overpic}
[width=\linewidth]{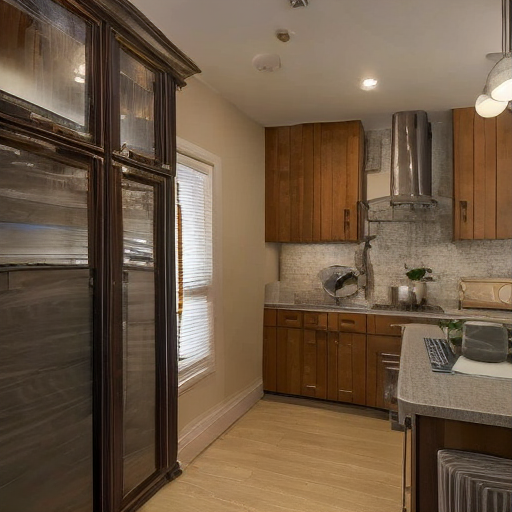}
\put(20,105){\small{Watermarked}}
\end{overpic}
\end{subfigure}
\hfill
\begin{subfigure}{0.16\textwidth}
\begin{overpic}
[width=\linewidth]{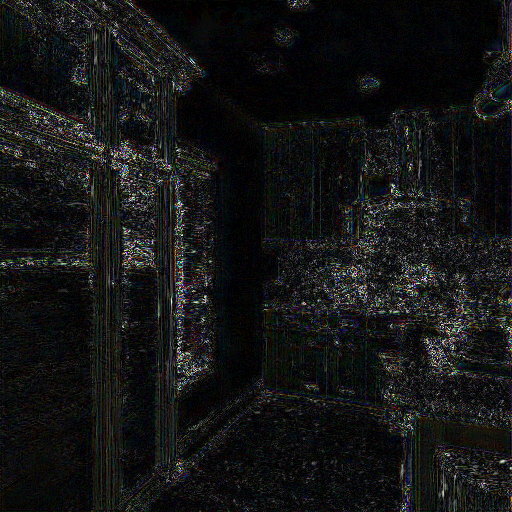}
\put(15, 105){\small{Pixel-wise ($\times$10)}}
\end{overpic}
\end{subfigure}

\begin{subfigure}{0.16\textwidth}
\begin{overpic}[width=\linewidth]{sec/fig/supp/sd/00597.png}
\put(-18,25){\rotatebox{90}{\small{WOUAF}}}
\end{overpic}
\end{subfigure}
\hfill
\begin{subfigure}{0.16\textwidth}
\includegraphics[width=\linewidth]{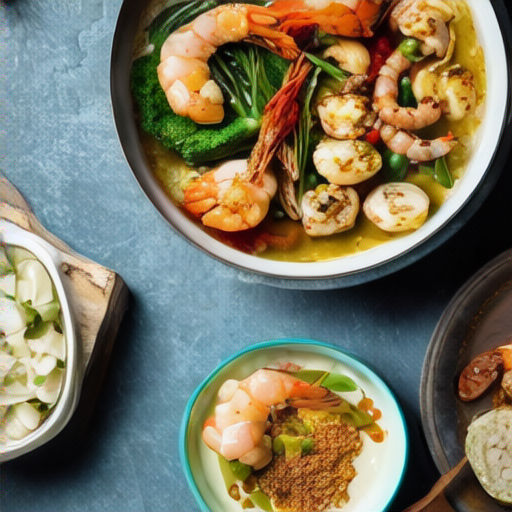}
\end{subfigure}
\hfill
\begin{subfigure}{0.16\textwidth}
\includegraphics[width=\linewidth]{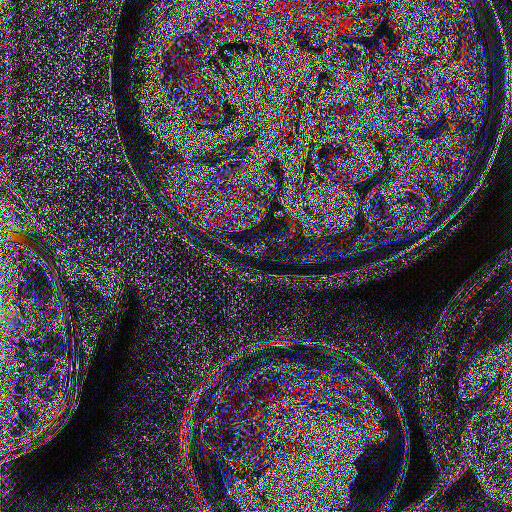}
\end{subfigure}
\hfill
\begin{subfigure}{0.16\textwidth}
\includegraphics[width=\linewidth]{sec/fig/supp/sd/00828.png}
\end{subfigure}
\hfill
\begin{subfigure}{0.16\textwidth}
\includegraphics[width=\linewidth]{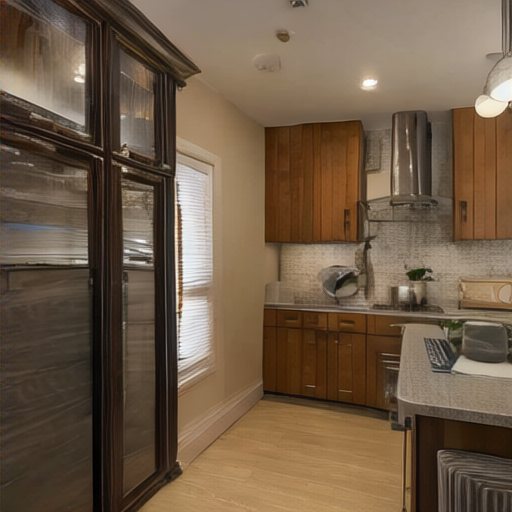}
\end{subfigure}
\hfill
\begin{subfigure}{0.16\textwidth}
\includegraphics[width=\linewidth]{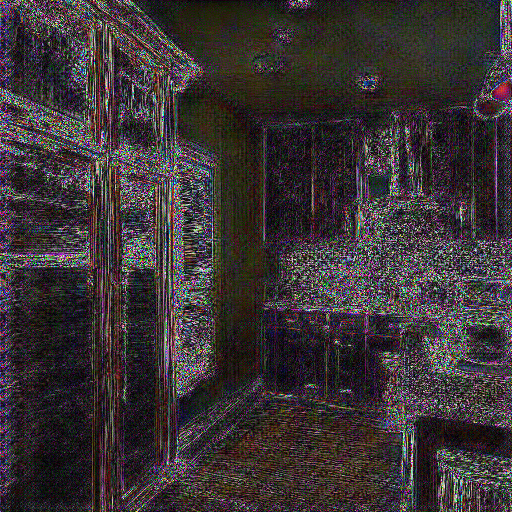}
\end{subfigure}

\begin{subfigure}{0.16\textwidth}
\begin{overpic}
[width=\linewidth]{sec/fig/supp/sd/00597.png}
\put(-18,10){\rotatebox{90}{\small{TEAWIB (ours)}}}
\end{overpic}
\end{subfigure}
\hfill
\begin{subfigure}{0.16\textwidth}
\includegraphics[width=\linewidth]{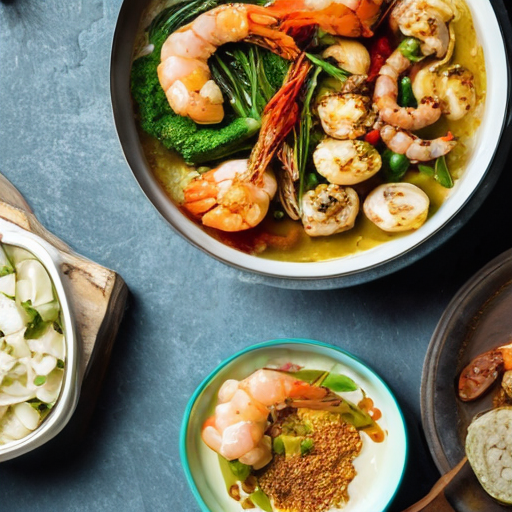}
\end{subfigure}
\hfill
\begin{subfigure}{0.16\textwidth}
\includegraphics[width=\linewidth]{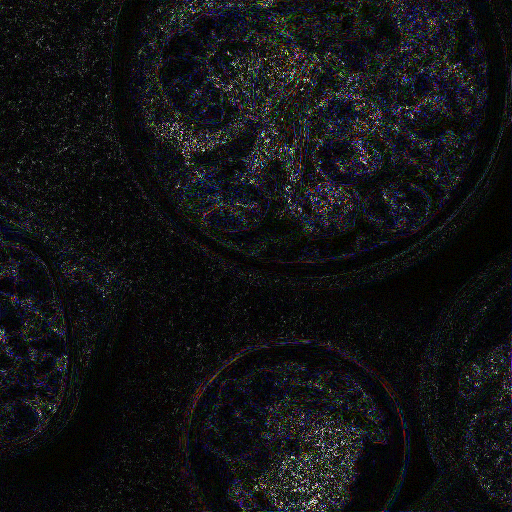}
\end{subfigure}
\hfill
\begin{subfigure}{0.16\textwidth}
\includegraphics[width=\linewidth]{sec/fig/supp/sd/00828.png}
\end{subfigure}
\hfill
\begin{subfigure}{0.16\textwidth}
\includegraphics[width=\linewidth]{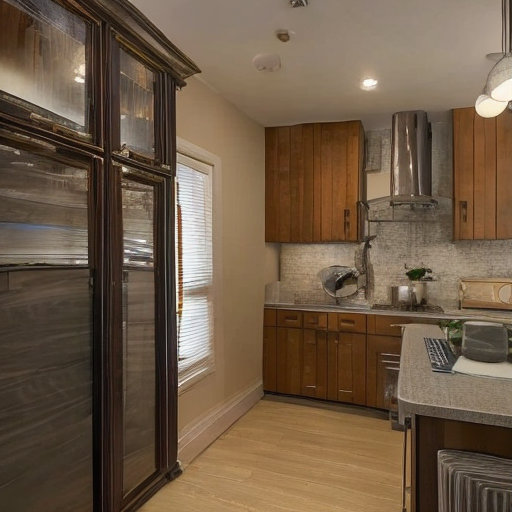}
\end{subfigure}
\hfill
\begin{subfigure}{0.16\textwidth}
\includegraphics[width=\linewidth]{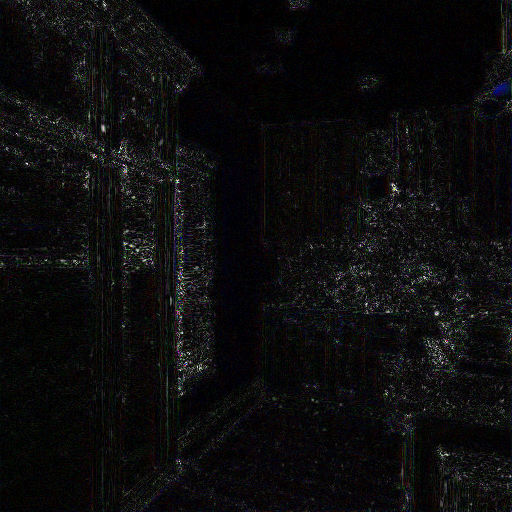}
\end{subfigure}
\caption{Qualitative comparison of TEAWIB with other ad-hoc watermark generation techniques on the MS-COCO validation set. Notably, our method preserves the high quality of the generated image and invisible watermark embedding.}
\label{fig:3}
\end{figure*}

\begin{figure*}
\centering
\vspace*{0.1cm}
\begin{subfigure}{0.16\textwidth}
\begin{overpic}[width=\linewidth]{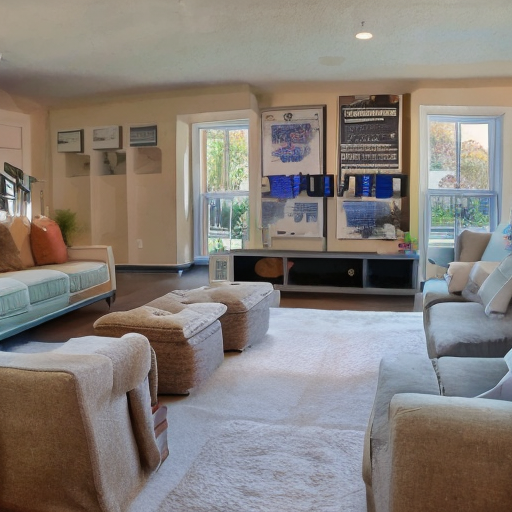}
\put(30,105){\small{Original}} % 文字在上方
\put(-18,40){\rotatebox{90}{\small{SG}}} % 文字在左侧
\end{overpic}
\end{subfigure}
\hfill
\begin{subfigure}{0.16\textwidth}
\begin{overpic}[width=\linewidth]{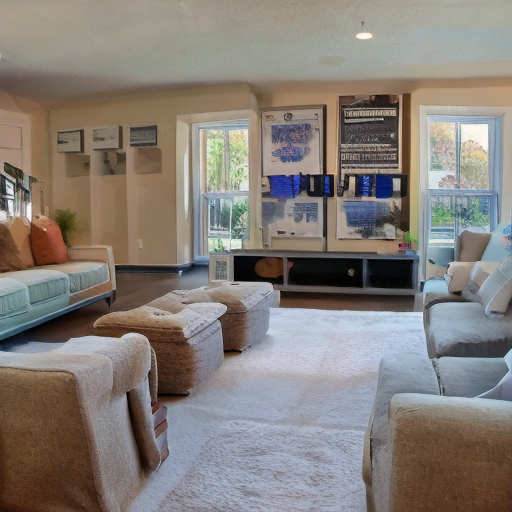}
\put(20,105){\small{Watermarked}}
\end{overpic}
\end{subfigure}
\hfill
\begin{subfigure}{0.16\textwidth}
\begin{overpic}[width=\linewidth]{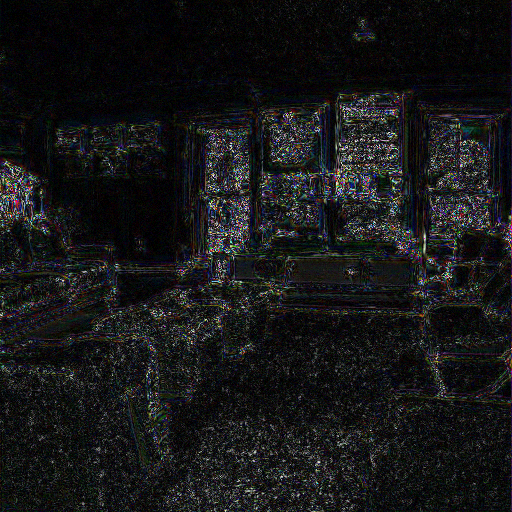}
\put(15, 105){\small{Pixel-wise ($\times$10)}}
\end{overpic}
\end{subfigure}
\hfill
\begin{subfigure}{0.16\textwidth}
\begin{overpic}
    [width=\linewidth]{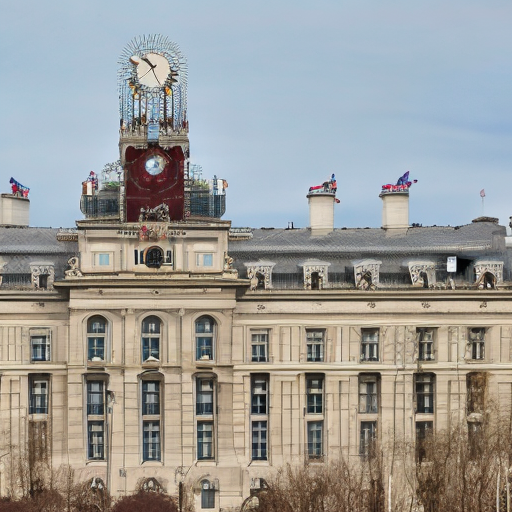}
\put(30,105){\small{Original}}
\end{overpic}
\end{subfigure}
\hfill
\begin{subfigure}{0.16\textwidth}
\begin{overpic}
[width=\linewidth]{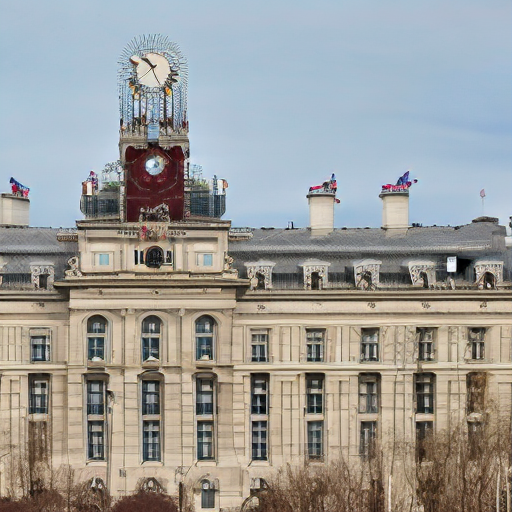}
\put(20,105){\small{Watermarked}}
\end{overpic}
\end{subfigure}
\hfill
\begin{subfigure}{0.16\textwidth}
\begin{overpic}
[width=\linewidth]{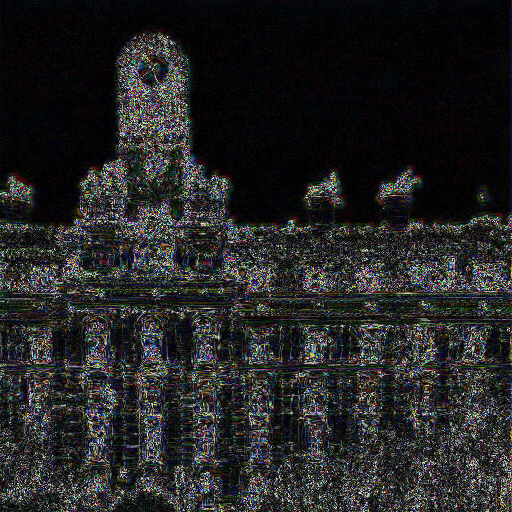}
\put(15, 105){\small{Pixel-wise ($\times$10)}}
\end{overpic}
\end{subfigure}

\begin{subfigure}{0.16\textwidth}
\begin{overpic}[width=\linewidth]{sec/fig/supp/sd/00829.png}
\put(-18,25){\rotatebox{90}{\small{WOUAF}}}
\end{overpic}
\end{subfigure}
\hfill
\begin{subfigure}{0.16\textwidth}
\includegraphics[width=\linewidth]{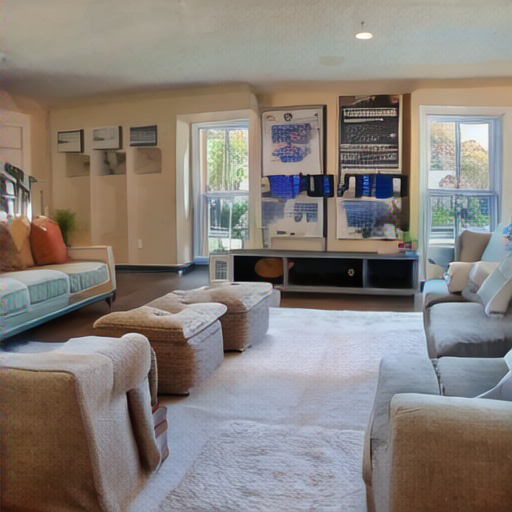}
\end{subfigure}
\hfill
\begin{subfigure}{0.16\textwidth}
\includegraphics[width=\linewidth]{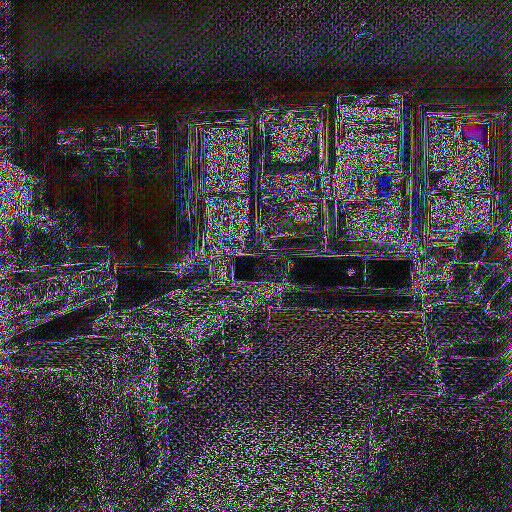}
\end{subfigure}
\hfill
\begin{subfigure}{0.16\textwidth}
\includegraphics[width=\linewidth]{sec/fig/supp/sd/00882.png}
\end{subfigure}
\hfill
\begin{subfigure}{0.16\textwidth}
\includegraphics[width=\linewidth]{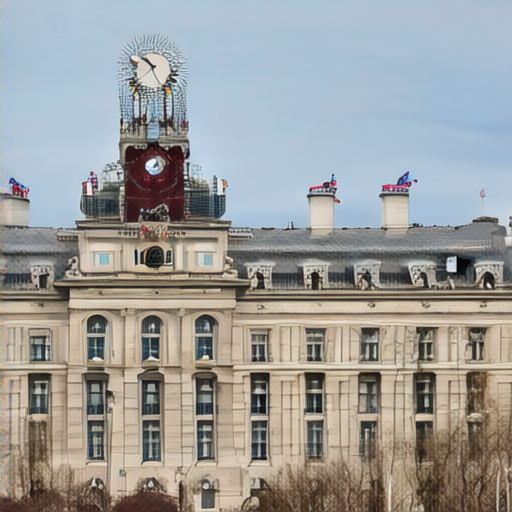}
\end{subfigure}
\hfill
\begin{subfigure}{0.16\textwidth}
\includegraphics[width=\linewidth]{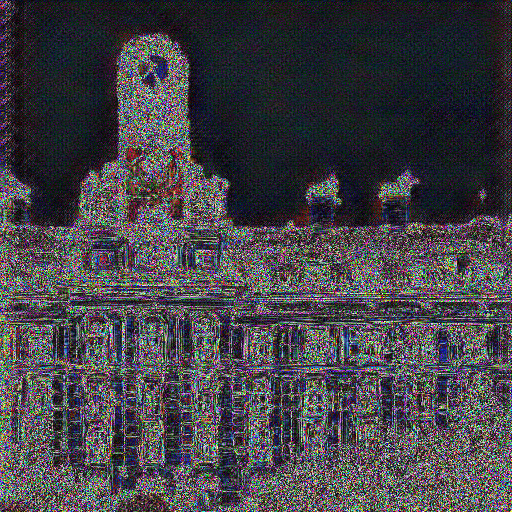}
\end{subfigure}

\begin{subfigure}{0.16\textwidth}
\begin{overpic}
[width=\linewidth]{sec/fig/supp/sd/00829.png}
\put(-18,10){\rotatebox{90}{\small{TEAWIB (ours)}}}
\end{overpic}
\end{subfigure}
\hfill
\begin{subfigure}{0.16\textwidth}
\includegraphics[width=\linewidth]{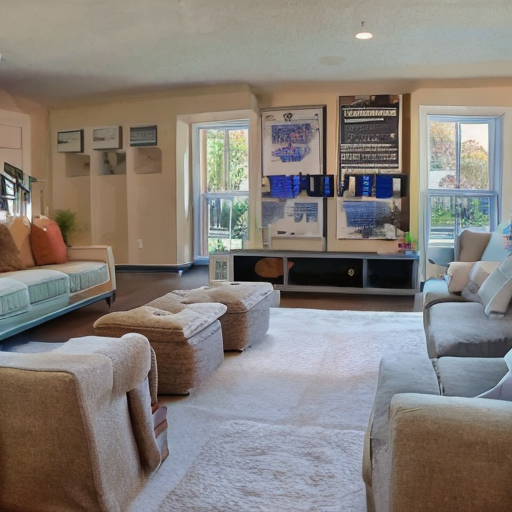}
\end{subfigure}
\hfill
\begin{subfigure}{0.16\textwidth}
\includegraphics[width=\linewidth]{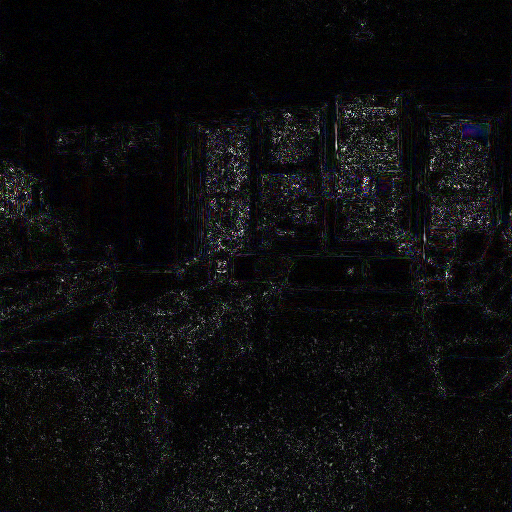}
\end{subfigure}
\hfill
\begin{subfigure}{0.16\textwidth}
\includegraphics[width=\linewidth]{sec/fig/supp/sd/00882.png}
\end{subfigure}
\hfill
\begin{subfigure}{0.16\textwidth}
\includegraphics[width=\linewidth]{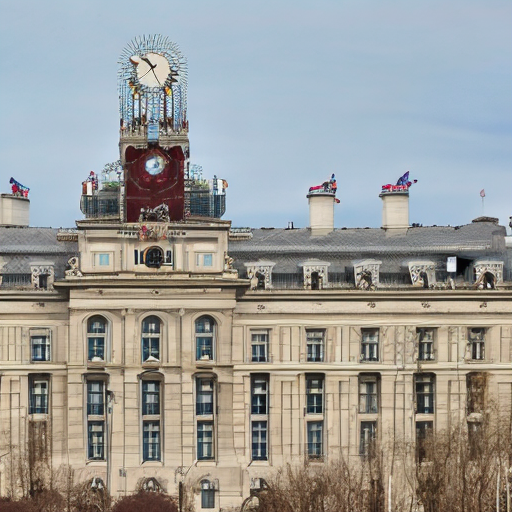}
\end{subfigure}
\hfill
\begin{subfigure}{0.16\textwidth}
\includegraphics[width=\linewidth]{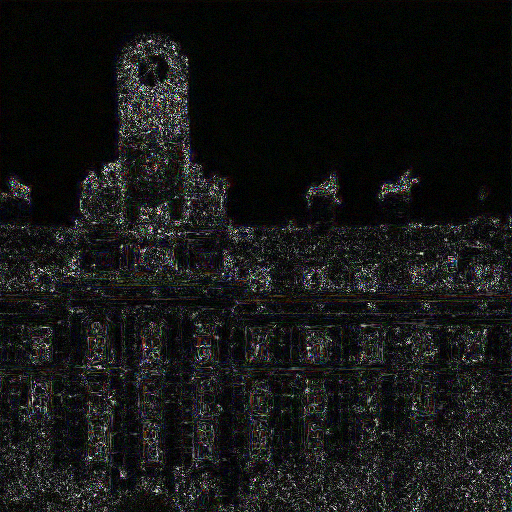}
\end{subfigure}
\caption{Qualitative comparison of TEAWIB with other ad-hoc watermark generation techniques on the MS-COCO validation set. Notably, our method preserves the high quality of the generated image and invisible watermark embedding.}
\label{fig:4}
\end{figure*}

\newpage
\begin{figure*}
\centering
\vspace*{0.1cm}
\begin{subfigure}{0.16\textwidth}
\begin{overpic}[width=\linewidth]{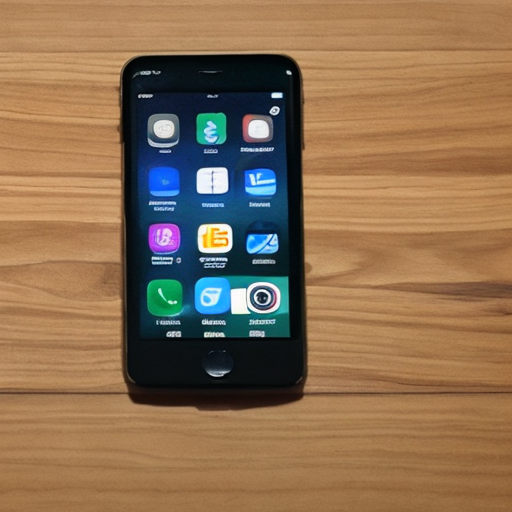}
\put(30,105){\small{Original}} % 文字在上方
\put(-18,40){\rotatebox{90}{\small{SG}}} % 文字在左侧
\end{overpic}
\end{subfigure}
\hfill
\begin{subfigure}{0.16\textwidth}
\begin{overpic}[width=\linewidth]{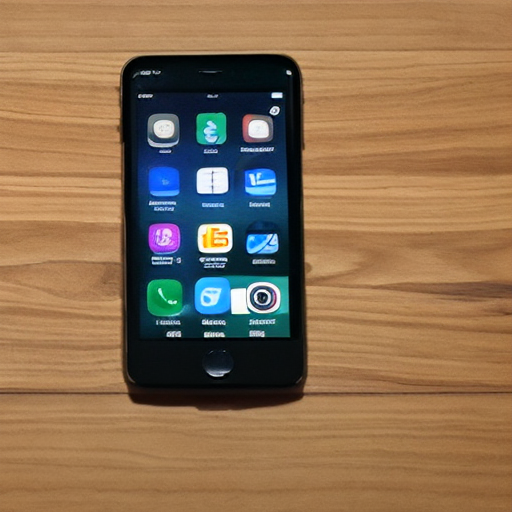}
\put(20,105){\small{Watermarked}}
\end{overpic}
\end{subfigure}
\hfill
\begin{subfigure}{0.16\textwidth}
\begin{overpic}[width=\linewidth]{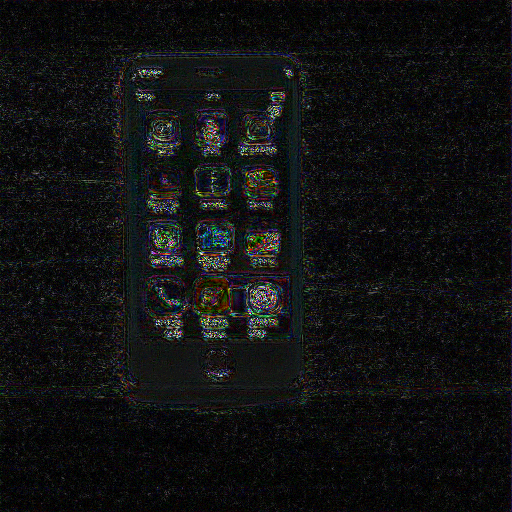}
\put(15, 105){\small{Pixel-wise ($\times$10)}}
\end{overpic}
\end{subfigure}
\hfill
\begin{subfigure}{0.16\textwidth}
\begin{overpic}
    [width=\linewidth]{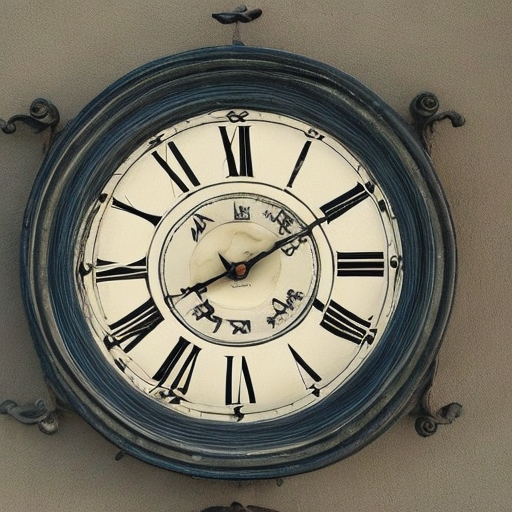}
\put(30,105){\small{Original}}
\end{overpic}
\end{subfigure}
\hfill
\begin{subfigure}{0.16\textwidth}
\begin{overpic}
[width=\linewidth]{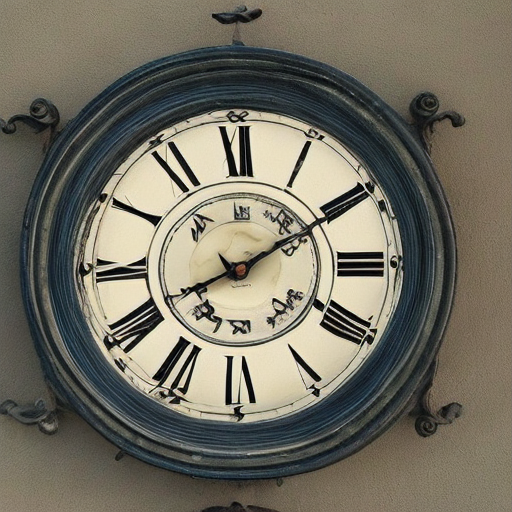}
\put(20,105){\small{Watermarked}}
\end{overpic}
\end{subfigure}
\hfill
\begin{subfigure}{0.16\textwidth}
\begin{overpic}
[width=\linewidth]{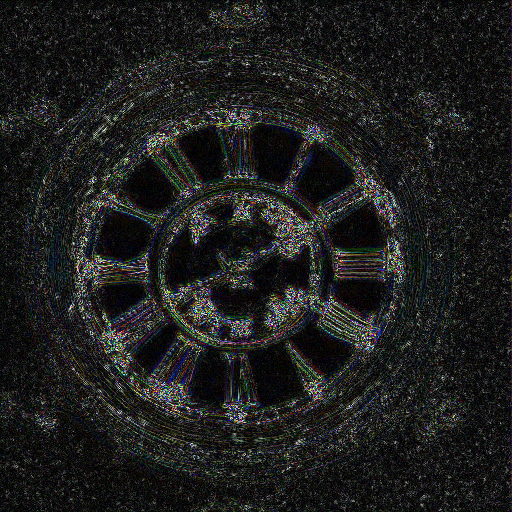}
\put(15, 105){\small{Pixel-wise ($\times$10)}}
\end{overpic}
\end{subfigure}

\begin{subfigure}{0.16\textwidth}
\begin{overpic}[width=\linewidth]{sec/fig/supp/sd/00959.png}
\put(-18,25){\rotatebox{90}{\small{WOUAF}}}
\end{overpic}
\end{subfigure}
\hfill
\begin{subfigure}{0.16\textwidth}
\includegraphics[width=\linewidth]{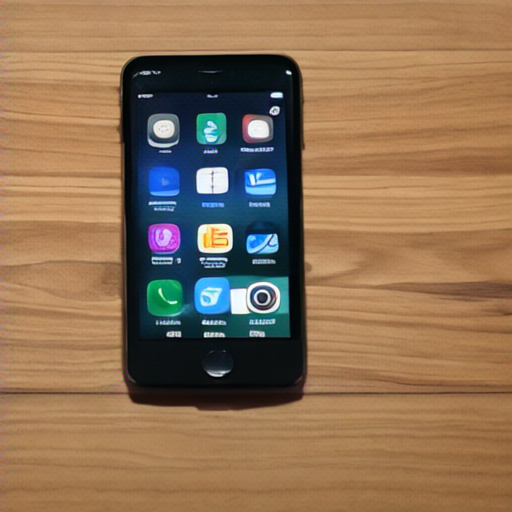}
\end{subfigure}
\hfill
\begin{subfigure}{0.16\textwidth}
\includegraphics[width=\linewidth]{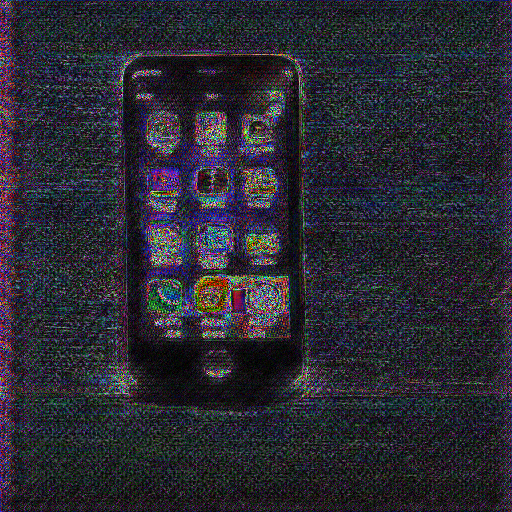}
\end{subfigure}
\hfill
\begin{subfigure}{0.16\textwidth}
\includegraphics[width=\linewidth]{sec/fig/supp/sd/00974.png}
\end{subfigure}
\hfill
\begin{subfigure}{0.16\textwidth}
\includegraphics[width=\linewidth]{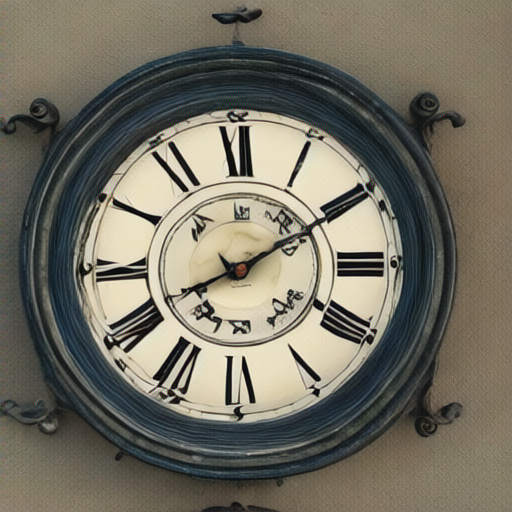}
\end{subfigure}
\hfill
\begin{subfigure}{0.16\textwidth}
\includegraphics[width=\linewidth]{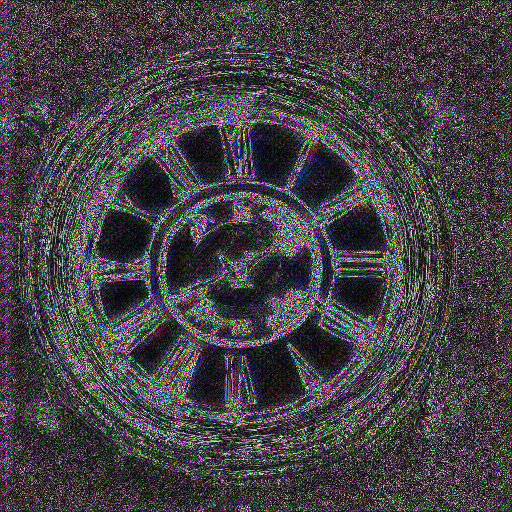}
\end{subfigure}

\begin{subfigure}{0.16\textwidth}
\begin{overpic}
[width=\linewidth]{sec/fig/supp/sd/00959.png}
\put(-18,10){\rotatebox{90}{\small{TEAWIB (ours)}}}
\end{overpic}
\end{subfigure}
\hfill
\begin{subfigure}{0.16\textwidth}
\includegraphics[width=\linewidth]{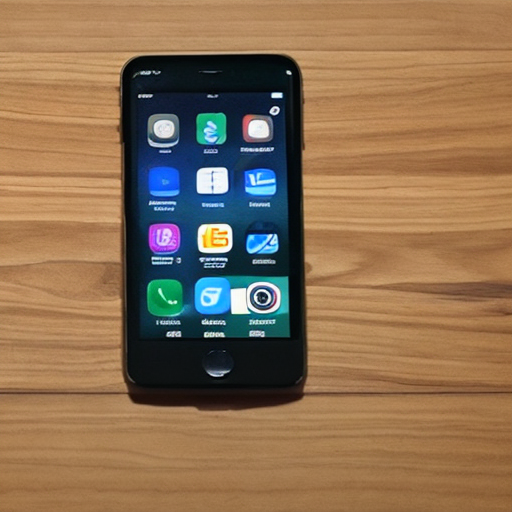}
\end{subfigure}
\hfill
\begin{subfigure}{0.16\textwidth}
\includegraphics[width=\linewidth]{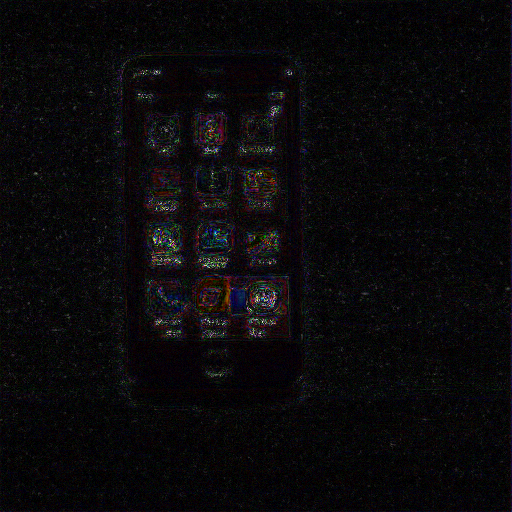}
\end{subfigure}
\hfill
\begin{subfigure}{0.16\textwidth}
\includegraphics[width=\linewidth]{sec/fig/supp/sd/00974.png}
\end{subfigure}
\hfill
\begin{subfigure}{0.16\textwidth}
\includegraphics[width=\linewidth]{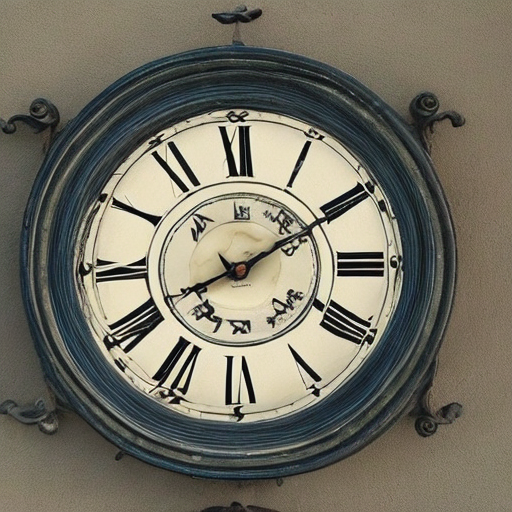}
\end{subfigure}
\hfill
\begin{subfigure}{0.16\textwidth}
\includegraphics[width=\linewidth]{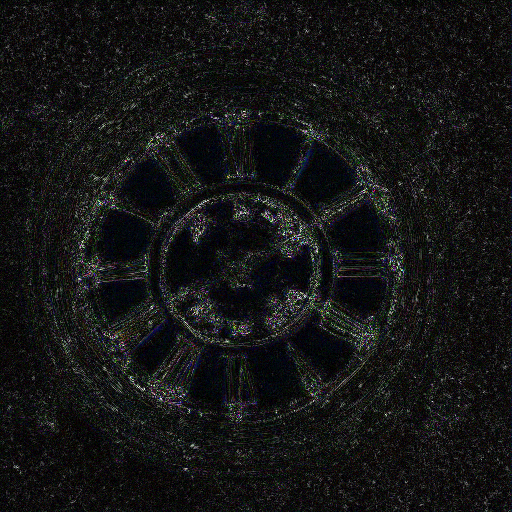}
\end{subfigure}
\caption{Qualitative comparison of TEAWIB with other ad-hoc watermark generation techniques on the MS-COCO validation set. Notably, our method preserves the high quality of the generated image and invisible watermark embedding.}
\label{fig:5}
\end{figure*}

\begin{figure*}
\centering
\vspace*{0.1cm}
\begin{subfigure}{0.16\textwidth}
\begin{overpic}[width=\linewidth]{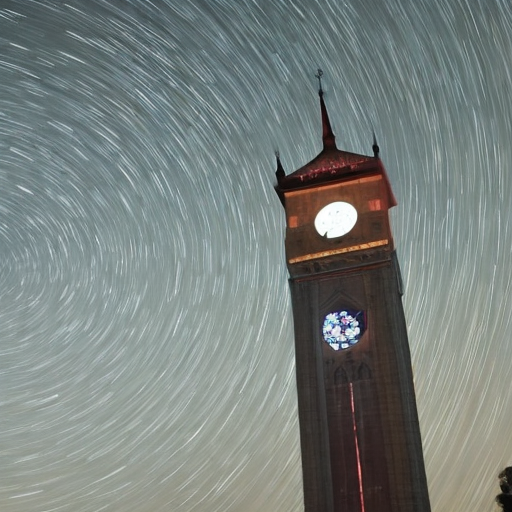}
\put(30,105){\small{Original}} % 文字在上方
\put(-18,40){\rotatebox{90}{\small{SG}}} % 文字在左侧
\end{overpic}
\end{subfigure}
\hfill
\begin{subfigure}{0.16\textwidth}
\begin{overpic}[width=\linewidth]{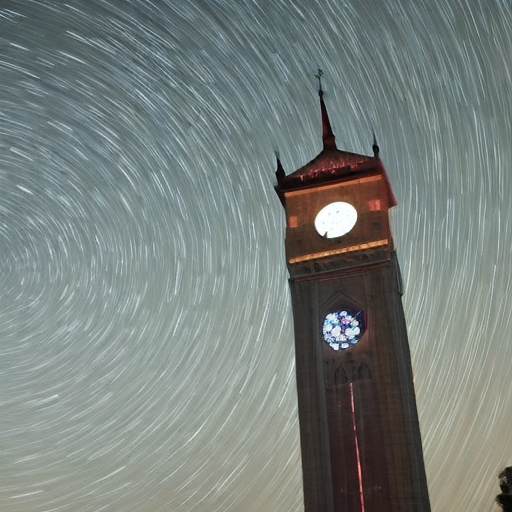}
\put(20,105){\small{Watermarked}}
\end{overpic}
\end{subfigure}
\hfill
\begin{subfigure}{0.16\textwidth}
\begin{overpic}[width=\linewidth]{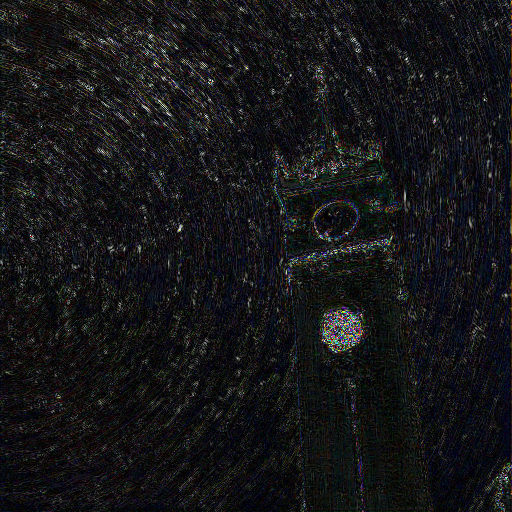}
\put(15, 105){\small{Pixel-wise ($\times$10)}}
\end{overpic}
\end{subfigure}
\hfill
\begin{subfigure}{0.16\textwidth}
\begin{overpic}
    [width=\linewidth]{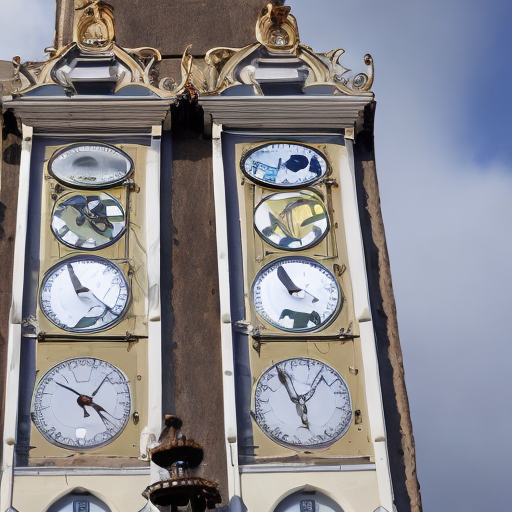}
\put(30,105){\small{Original}}
\end{overpic}
\end{subfigure}
\hfill
\begin{subfigure}{0.16\textwidth}
\begin{overpic}
[width=\linewidth]{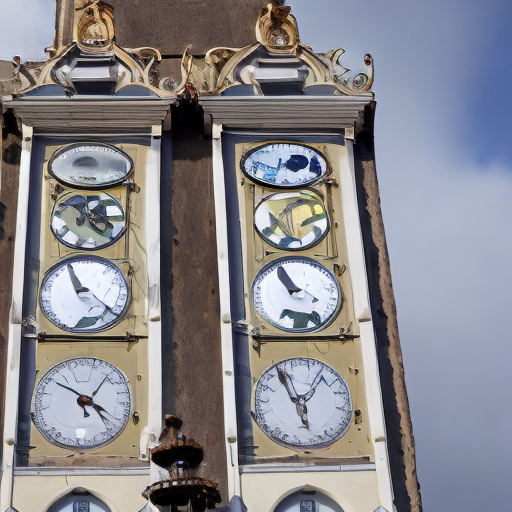}
\put(20,105){\small{Watermarked}}
\end{overpic}
\end{subfigure}
\hfill
\begin{subfigure}{0.16\textwidth}
\begin{overpic}
[width=\linewidth]{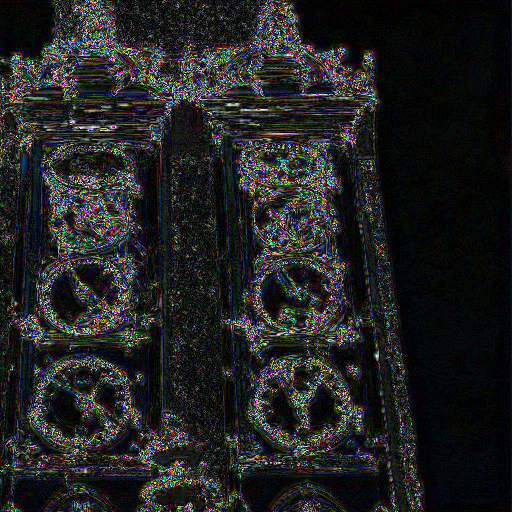}
\put(15, 105){\small{Pixel-wise ($\times$10)}}
\end{overpic}
\end{subfigure}

\begin{subfigure}{0.16\textwidth}
\begin{overpic}[width=\linewidth]{sec/fig/supp/sd/00991.png}
\put(-18,25){\rotatebox{90}{\small{WOUAF}}}
\end{overpic}
\end{subfigure}
\hfill
\begin{subfigure}{0.16\textwidth}
\includegraphics[width=\linewidth]{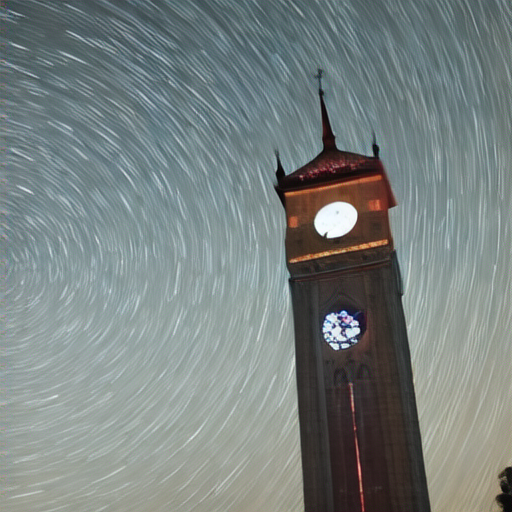}
\end{subfigure}
\hfill
\begin{subfigure}{0.16\textwidth}
\includegraphics[width=\linewidth]{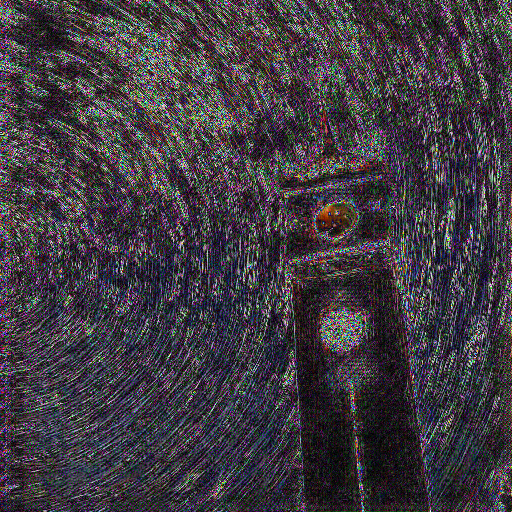}
\end{subfigure}
\hfill
\begin{subfigure}{0.16\textwidth}
\includegraphics[width=\linewidth]{sec/fig/supp/sd/00997.png}
\end{subfigure}
\hfill
\begin{subfigure}{0.16\textwidth}
\includegraphics[width=\linewidth]{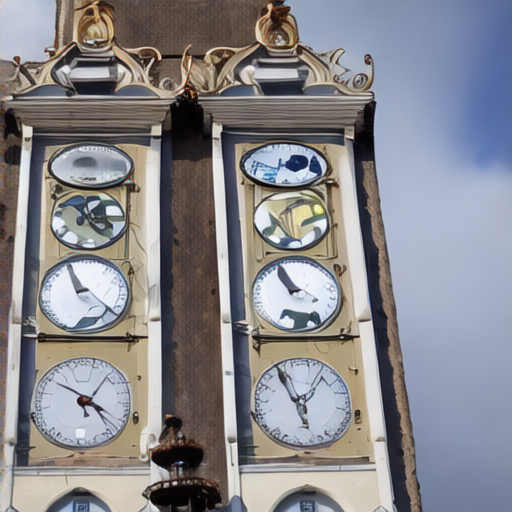}
\end{subfigure}
\hfill
\begin{subfigure}{0.16\textwidth}
\includegraphics[width=\linewidth]{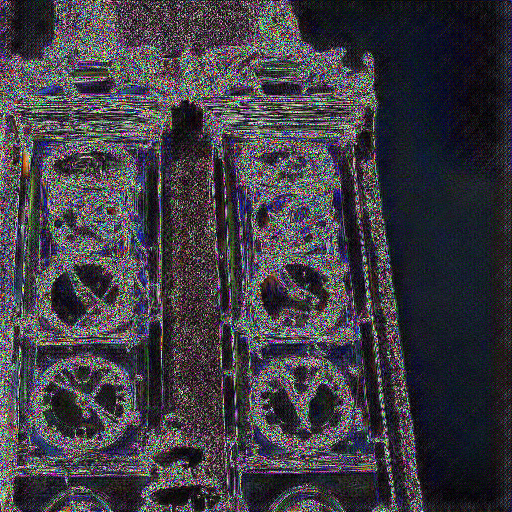}
\end{subfigure}

\begin{subfigure}{0.16\textwidth}
\begin{overpic}
[width=\linewidth]{sec/fig/supp/sd/00991.png}
\put(-18,10){\rotatebox{90}{\small{TEAWIB (ours)}}}
\end{overpic}
\end{subfigure}
\hfill
\begin{subfigure}{0.16\textwidth}
\includegraphics[width=\linewidth]{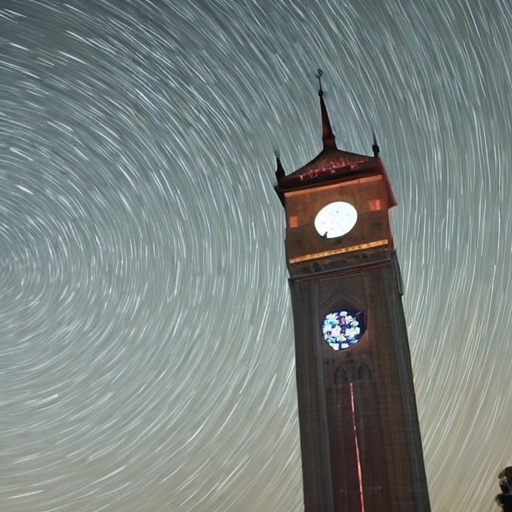}
\end{subfigure}
\hfill
\begin{subfigure}{0.16\textwidth}
\includegraphics[width=\linewidth]{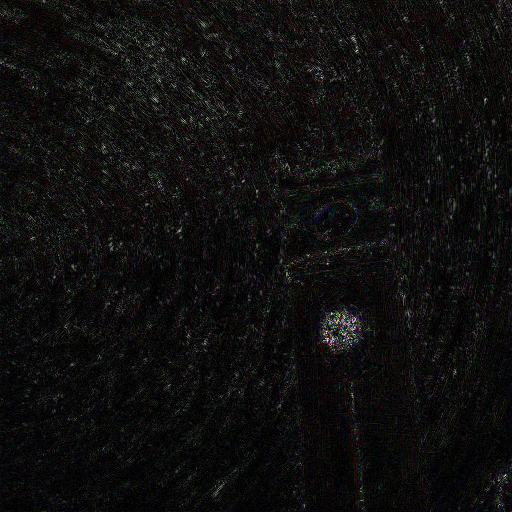}
\end{subfigure}
\hfill
\begin{subfigure}{0.16\textwidth}
\includegraphics[width=\linewidth]{sec/fig/supp/sd/00997.png}
\end{subfigure}
\hfill
\begin{subfigure}{0.16\textwidth}
\includegraphics[width=\linewidth]{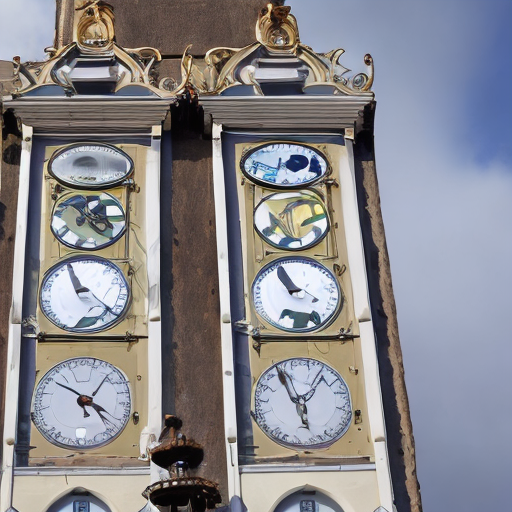}
\end{subfigure}
\hfill
\begin{subfigure}{0.16\textwidth}
\includegraphics[width=\linewidth]{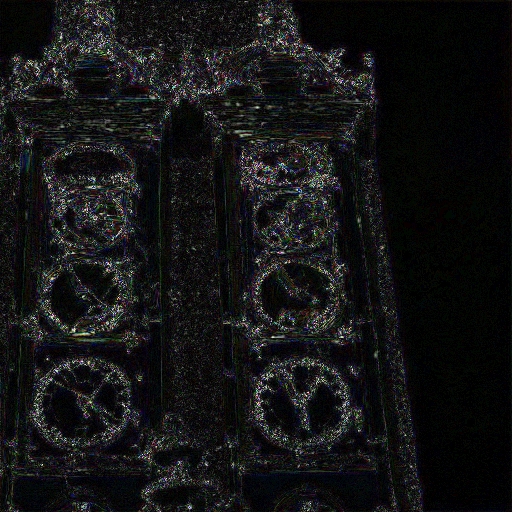}
\end{subfigure}
\caption{Qualitative comparison of TEAWIB with other ad-hoc watermark generation techniques on the MS-COCO validation set. Notably, our method preserves the high quality of the generated image and invisible watermark embedding.}
\label{fig:6}
\end{figure*}
% \newpage

\begin{figure*}

\vspace*{0.1cm}
\begin{minipage}[b]{\textwidth}
\begin{subfigure}{0.16\textwidth}
\begin{overpic}[width=\linewidth]{sec/fig/supp/sd/00807.png}
\put(30,105){\small{Original}} % 文字在上方
\put(-18,40){\rotatebox{90}{\small{SG}}} % 文字在左侧
\end{overpic}
\end{subfigure}
\hfill
\begin{subfigure}{0.16\textwidth}
\begin{overpic}[width=\linewidth]{sec/fig/supp/sg/00807.png}
\put(20,105){\small{Watermarked}}
\end{overpic}
\end{subfigure}
\hfill
\begin{subfigure}{0.16\textwidth}
\begin{overpic}[width=\linewidth]{sec/fig/supp/sg/diff_00807.png}
\put(15, 105){\small{Pixel-wise ($\times$10)}}
\end{overpic}
\end{subfigure}
\hfill
\begin{subfigure}{0.16\textwidth}
\begin{overpic}
    [width=\linewidth]{sec/fig/supp/sd/00931.png}
\put(30,105){\small{Original}}
\end{overpic}
\end{subfigure}
\hfill
\begin{subfigure}{0.16\textwidth}
\begin{overpic}
[width=\linewidth]{sec/fig/supp/sg/00931.png}
\put(20,105){\small{Watermarked}}
\end{overpic}
\end{subfigure}
\hfill
\begin{subfigure}{0.16\textwidth}
\begin{overpic}
[width=\linewidth]{sec/fig/supp/sg/diff_00931.png}
\put(15, 105){\small{Pixel-wise ($\times$10)}}
\end{overpic}
\end{subfigure}

\begin{subfigure}{0.16\textwidth}
\begin{overpic}[width=\linewidth]{sec/fig/supp/sd/00807.png}
\put(-18,25){\rotatebox{90}{\small{WOUAF}}}
\end{overpic}
\end{subfigure}
\hfill
\begin{subfigure}{0.16\textwidth}
\includegraphics[width=\linewidth]{sec/fig/supp/wouaf/00807.png}
\end{subfigure}
\hfill
\begin{subfigure}{0.16\textwidth}
\includegraphics[width=\linewidth]{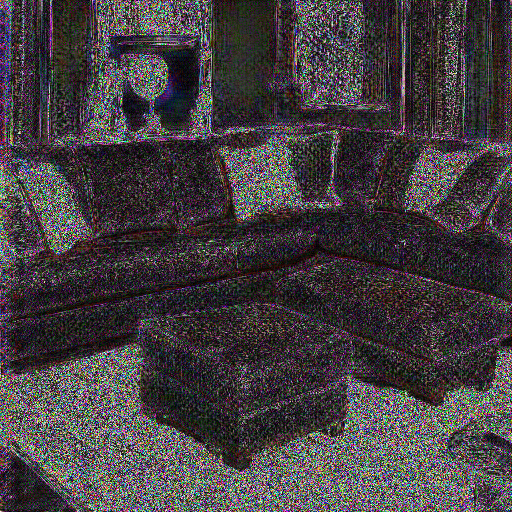}
\end{subfigure}
\hfill
\begin{subfigure}{0.16\textwidth}
\includegraphics[width=\linewidth]{sec/fig/supp/sd/00931.png}
\end{subfigure}
\hfill
\begin{subfigure}{0.16\textwidth}
\includegraphics[width=\linewidth]{sec/fig/supp/wouaf/00931.png}
\end{subfigure}
\hfill
\begin{subfigure}{0.16\textwidth}
\includegraphics[width=\linewidth]{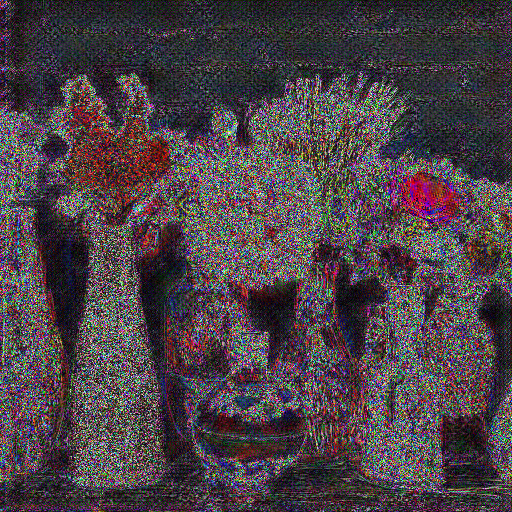}
\end{subfigure}

\begin{subfigure}{0.16\textwidth}
\begin{overpic}
[width=\linewidth]{sec/fig/supp/sd/00807.png}
\put(-18,10){\rotatebox{90}{\small{TEAWIB (ours)}}}
\end{overpic}
\end{subfigure}
\hfill
\begin{subfigure}{0.16\textwidth}
\includegraphics[width=\linewidth]{sec/fig/supp/teawib/00807.png}
\end{subfigure}
\hfill
\begin{subfigure}{0.16\textwidth}
\includegraphics[width=\linewidth]{sec/fig/supp/teawib/diff_00807.png}
\end{subfigure}
\hfill
\begin{subfigure}{0.16\textwidth}
\includegraphics[width=\linewidth]{sec/fig/supp/sd/00931.png}
\end{subfigure}
\hfill
\begin{subfigure}{0.16\textwidth}
\includegraphics[width=\linewidth]{sec/fig/supp/teawib/00931.png}
\end{subfigure}
\hfill
\begin{subfigure}{0.16\textwidth}
\includegraphics[width=\linewidth]{sec/fig/supp/teawib/diff_00931.png}
\end{subfigure}
\caption{Qualitative comparison of TEAWIB with other ad-hoc watermark generation techniques on the MS-COCO validation set. Notably, our method preserves the high quality of the generated image and invisible watermark embedding.}
\label{fig:7}
\end{minipage}

\vspace{10mm}
\begin{minipage}[t]{0.5\textwidth}

{\small
    \bibliographystyle{ieeenat_fullname}
    \bibliography{main}
}
\end{minipage}
\end{figure*}
